# Supplementary material for: CHAMELEON: A Deep Learning Meta-Architecture for News Recommender Systems [Phd. Thesis]
Source: arXiv:2001.04831 source file (2019-12-29)
Supplement: Supplementary file 1 [file cap3-additionalrefs.tex]

\section{Additional readings}

\subsection{What to Do Next: Modeling User Behaviors by Time-LSTM}
TODO: Desenvolver de \cite{zhunext2017}

Recently, Recurrent Neural Network (RNN) solutions
for recommender systems (RS) are becoming
increasingly popular. The insight is that, there exist
some intrinsic patterns in the sequence of users’
actions, and RNN has been proved to perform excellently
when modeling sequential data. In traditional
tasks such as language modeling, RNN solutions
usually only consider the sequential order
of objects without the notion of interval. However,
in RS, time intervals between users’ actions are of
significant importance in capturing the relations of
users’ actions and the traditional RNN architectures
are not good at modeling them. In this paper, we
propose a new LSTM variant, i.e. Time-LSTM,
to model users’ sequential actions. Time-LSTM
equips LSTM with time gates to model time intervals.
These time gates are specifically designed,
so that compared to the traditional RNN solutions,
Time-LSTM better captures both of users’ shortterm
and long-term interests, so as to improve the
recommendation performance. Experimental results
on two real-world datasets show the superiority
of the recommendation method using TimeLSTM
over the traditional methods.

%Code using Theano: https://github.com/DarryO/time_lstm

\subsection{Recurrent coevolutionary latent feature processes for continuous-time recommendation}
Desenvolver de \cite{dai2016recurrent}

Matching users to the right items at the right time is a fundamental task in recommender systems. As users interact with different items over time, users' and items' feature may drift, evolve and co-evolve over time. Traditional models based on static latent features or discretizing time into epochs can become ineffective for capturing the fine-grained temporal dynamics in the user-item interactions. We propose a coevolutionary latent feature process model that accurately captures the coevolving nature of users' and items' feature. We use a recurrent neural network to automatically learn a representation of influences from drift, evolution and co-evolution of user and item features. We develop an efficient stochastic gradient algorithm for learning the model parameters which can readily scale up to millions of events. Experiments on diverse real-world datasets demonstrate significant improvements in user behavior prediction compared to state-of-the-arts.

\subsection{Deep Coevolutionary Network: Embedding User and Item Features for Recommendation}
TODO: Desenvolver de \cite{dai2017deep}

Recommender systems o=en use latent features to explain the behaviors
of users and capture the properties of items. As users
interact with dierent items over time, user and item features can
in=uence each other, evolve and co-evolve over time. e compatibility
of user and item’s feature further in=uence the future
interaction between users and items.
Recently, point process based models have been proposed in
the literature aiming to capture the temporally evolving nature of
these latent features. However, these models o=en make strong
parametric assumptions about the evolution process of the user
and item latent features, which may not re=ect the reality, and has
limited power in expressing the complex and nonlinear dynamics
underlying these processes.
To address these limitations, we propose a novel deep coevolutionary
network model (DeepCoevolve), for learning user and
item features based on their interaction graph. DeepCoevolve use
recurrent neural network (RNN) over evolving networks to de=ne
the intensity function in point processes, which allows the model
to capture complex mutual in=uence between users and items, and
the feature evolution over time. We also develop an ecient procedure
for training the model parameters, and show that the learned
models lead to signi=cant improvements in recommendation and activity
prediction compared to previous state-of-the-arts parametric
models.

\subsection{Temporal learning and sequence modeling for a job recommender system}
TODO: Desenvolver de \cite{liu2016temporal}

We present our solution to the job recommendation task for RecSys Challenge 2016. The main contribution of our work is to combine temporal learning with sequence modeling to capture complex user-item activity patterns to improve job recommendations. First, we propose a time-based ranking model applied to historical observations and a hybrid matrix factorization over time re-weighted interactions. Second, we exploit sequence properties in user-items activities and develop a RNN-based recommendation model. Our solution achieved 5th place in the challenge among more than 100 participants. Notably, the strong performance of our RNN approach shows a promising new direction in employing sequence modeling for recommendation systems.

\subsection{Click-Through Rate prediction}

\subsubsection{Wide \& Deep Learning for Recommender Systems}
TODO: Desenvolver de \cite{cheng2016wide}

\subsubsection{DeepFM: A Factorization-Machine based Neural Network for CTR Prediction}
TODO: Desenvolver de \cite{guo2017deepfm}
%Tensorflow code: https://github.com/Leavingseason/OpenLearning4DeepRecsys

%%%%%%%%%%%%%%%%%%%%%%%%%%%%%%%%%%%%%%%%%%%%%%%

Refugo do Cap 3

\subsection{From Word Embeddings to Item Recommendation}

TODO: Summarize from \cite{ozsoy2016} (ver resumo docs)

\subsection{Word embedding based retrieval model for similar cases recommendation}

TODO: Summarize from \cite{zhao2015word}

\subsection{Restricted Boltzman Machines for Collaborative Filtering}

Early pioneer work which used neural network was done in \cite{salakhutdinov2007}. They introduced a two-layer Restricted Boltzmann Machines (RBM) to model ratings. Since maximum likelihood estimation is intractable in these models, they show that optimization can be done efficiently by following an approximation to the gradient of a different objective function \cite{zheng2016}. 

A RBM model is trained for each user, and the visible softmax units corresponds with the items rated by the user, as shown in Figure \ref{figure:rbmarch}. If user \textit{a} and user \textit{b} rated the same item, their RBMs share weights connected to the corresponding visible unit \cite{zheng2016}. This consists in an advantage for computational tractability.

\begin{figure}[h]
	\centering
	\includegraphics[height=7cm]{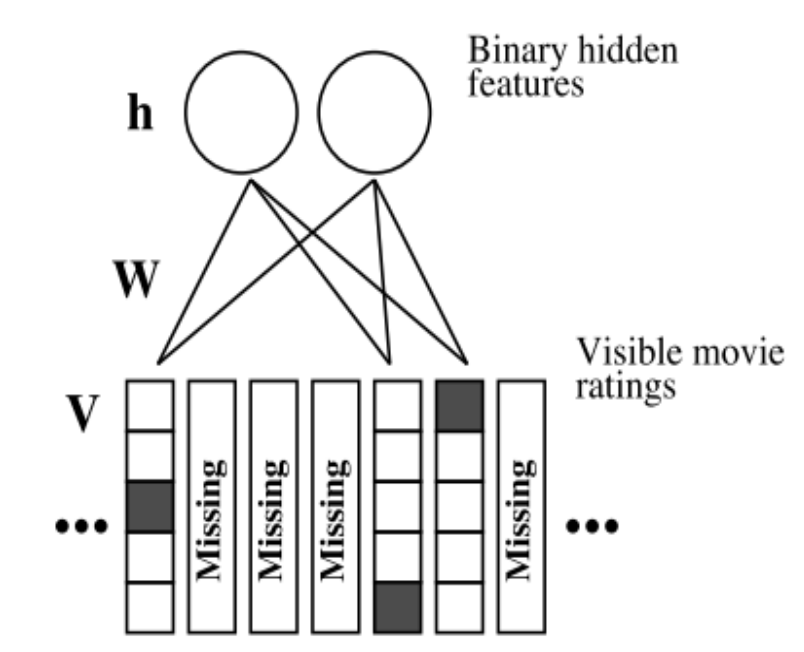}
	\caption{Architecture of a RBM for a user \cite{zheng2016}}
	\label{figure:rbmarch}
\end{figure}

Although the authors in \cite{salakhutdinov2007} show that RBM can be successfully applied to the recommendation problem and slightly outperforms traditional Matrix Factorization, the proposed model is not deep enough and only consists of 2 layers. Learning deep models has been successfully applied in the domain of modeling temporal data \cite{bengio2003} \cite{pan2008} and learning word embedding \cite{mikolov2013} \cite{turian2010}. Training a deeper RBM is helpful for capturing hierarchical latent factors of users and items and more accurately modeling ratings \cite{zheng2016}.

RBM does not make use of content information, such as user profiles or review texts \cite{zheng2016}. As a result, the proposed model cannot deal with the cold start problem \cite{schein2002}, where recommender systems are required to give recommendations to novel users who have no preference on any items, or recommending items that no user of the community has rated yet  \cite{zheng2016}. 

RBM targets rating prediction, not top-N recommendation, and its loss function considers only the observed ratings. It is technically challenging to incorporate negative sampling, which would be required for top-N recommendation, into the training of RBM. For this reason, we do not compare with RBM in our experiments, but test several other neural network baselines that work for top-N recommendation \cite{wu2016}.

\subsection{Autoencoders for recommendation}

Recently autoencoders have become a popular choice for building recommendation systems \cite{chen2012}\cite{sedhain2015}\cite{strub2015}. The idea of user-based AutoRec \cite{sedhain2015} is to learn hidden structures that can reconstruct a user's ratings given her historical ratings as inputs. In terms of user personalization, this approach shares a similar spirit as the item-item model \cite{ning2011}\cite{sarwar2001} that represent a user as her rated item features. While previous work has lent support for addressing collaborative filtering, most of them have focused on observed ratings and modeled the observed data only. As a result, they can easily fail to learn users preference from the positive-only implicit data.

A subclass of deep CF methods use denoising autoencoders as the central component of their model, as can be seeing in this section.

To utilize information from text, \cite{wang2015} integrates an autoencoder and Probabilistic Matrix Factorization (PMF). Item text is represented by using bag-of-words and taken as input to the autoencoder to learn item features. User features are modeled by a Gaussian distribution. However, they do not jointly model users and items from text. In addition, this approach is only suitable for one-class collaborative filtering problems \cite{pan2008} \cite{zheng2016} 

\subsubsection{Collaborative Deep Learning (CDL)}.
In \cite{wang2015}, it was introduced a technique named Collaborative Deep Learning (CDL), which utilizes review texts along with ratings, in order to address the cold start problem. They integrate a bayesian Stack Denoise Auto Encoder (SDAE) \cite{vincent2010} and Collaborative Topic Regression (CTR) \cite{wang2011}. It learns latent factors of items from review texts and draw a latent user vector from Gaussian distribution \cite{zheng2016}. CDL uses tags and metadata instead of the item ID. CDL was the first deep model to learn from review texts for recommender systems \cite{betru2017}.

In \cite{zheng2016}, some critiques for the work of \cite{wang2015} are presented. First, Collaborative Deep Learning only models item review texts. In recommender systems, user provides reviews to express their feelings. These review texts can be utilized to learn preference of users. 

Second, review texts are represented by using bag of words scheme. As we know, bag of words vectors only convey the frequency of words. If two reviews are semantically related but use different words, CDL, which uses bag-of-words, may not consider the two reviews to be similar . The vocabulary in English is very diverse and two reviews can be semantically similar even with low lexical overlap, so semantic meaning is especially important \cite{zheng2016}. However, semantic meanings, which are essential for reveal user attitudes and item properties, are lost in CDL. 

At last, in Collaborative Deep Learning, word order is ignored. However, in many text modeling applications, word order is extremely important \cite{wallach2006}. To further improve the performance of Collaborative Deep Learning, word order should be taken into consideration while modeling review texts \cite{betru2017}.

\subsection{Deep collaborative filtering via marginalized denoising auto-encoder}

In \cite{li2015deep}, authors propose a general deep architecture named Deep Collaborative Filtering (DCF), shown in Figure \ref{figure:dcf}, which integrates matrix factorization and deep feature learning. It models the mappings between the latent factors used in CF and the latent layers in deep models.
They also present a practical instantiation of the proposed architecture, by utilizing the probabilistic matrix factorization and Marginalized Denoising Auto-encoders (mDA) \cite{chen2012}. The scalability and low computational cost of the mDA makes it an interesting approach.

Unlike \cite{wang2015} which integrates collaborative topic regression and bayesian stacked denoising auto-encoders and requires learning of a large number of hyper parameters using an EM style algorithm, their approach uses a ore efficient architecture based upon mDA and stochastic gradient descent and is more computationally efficient and scalable.

\begin{figure}[h]
	\centering
	\includegraphics[height=7cm]{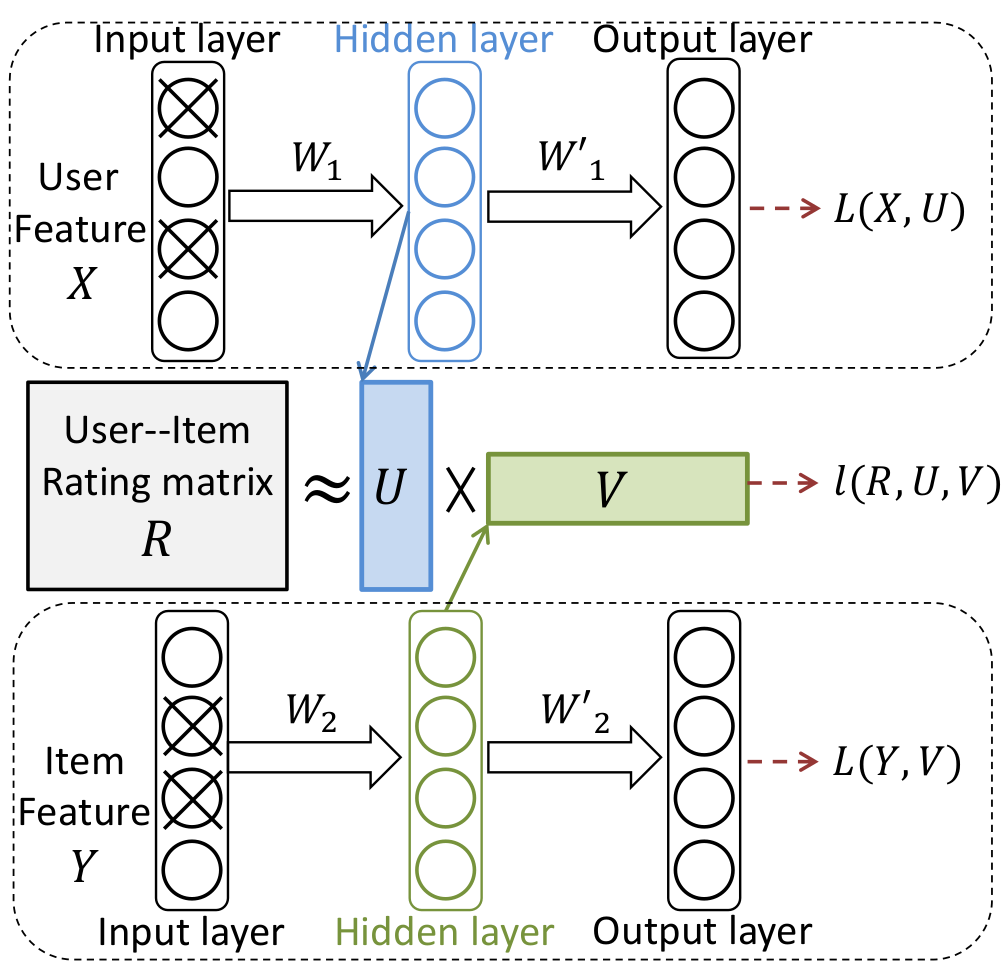}
	\caption{DCF general framework in \cite{li2015deep}}
	\label{figure:dcf}
\end{figure}

\subsubsection{Collaborative filtering with stacked denoising autoencoders and sparse inputs}
TODO:Summarize from \cite{strub2015}

\subsubsection{Collaborative topic modeling for recommending scientific articles}
TODO:Summarize from \cite{wang2011}

From \cite{wu2016}...
Another related work is [27], which also uses the Auto-Encoder
for recommender systems. This work studies the particular prob-
lem of article recommendation, and improves the well-known model
Collaborative Topic Regression [26] by replacing its Topic Model
component by a Bayesian Auto-Encoder, which is used for learn-
ing the latent feature representations for the articles. Different from
this model, our model is a generic model and addresses the general
top-N recommendation problem, and the inputs are user behaviors
instead of item/article features.

\subsubsection{Autorec: Autoencoders meet collaborative filtering}
TODO: Summarize from \cite{sedhain2015}

From \cite{wu2016}...
We are aware of a concurrent proposal called AutoRec [20],
which uses the Auto-Encoder for rating prediction. The main dif-
ferences are as follows: 1) AutoRec only considers the observed
ratings in the loss function, which does not guarantee the perfor-
mance for top-N recommendation. 2) They use the vanilla Auto-
Encoder structure, while we prove that introducing user factors in
the model can greatly improve performance. 3) AutoRec does not
employ the denoising technique, which is a major part of our work.

\subsubsection{Collaborative Denoising Auto-Encoders for top-n recommender systems (CDAE)}

Learning from intentionally corrupted input has been widely studied. In \cite{wu2016}, a method for top-N recommendation named Collaborative Denoising Auto-Encoder (CDAE) is presented. It is probably the first work to utilize, for recommender systems, the idea of Denoising Auto-Encoders (DAE) \cite{vincent2008extracting}. DAE extends the classical auto-encoder by training to reconstruct each data point x from its (partially) corrupted version. The goal of DAE is to force the hidden layer to discover more robust features and to prevent it from simply learning the identity function.

\begin{figure}[h]
	\centering
	\includegraphics[height=7cm]{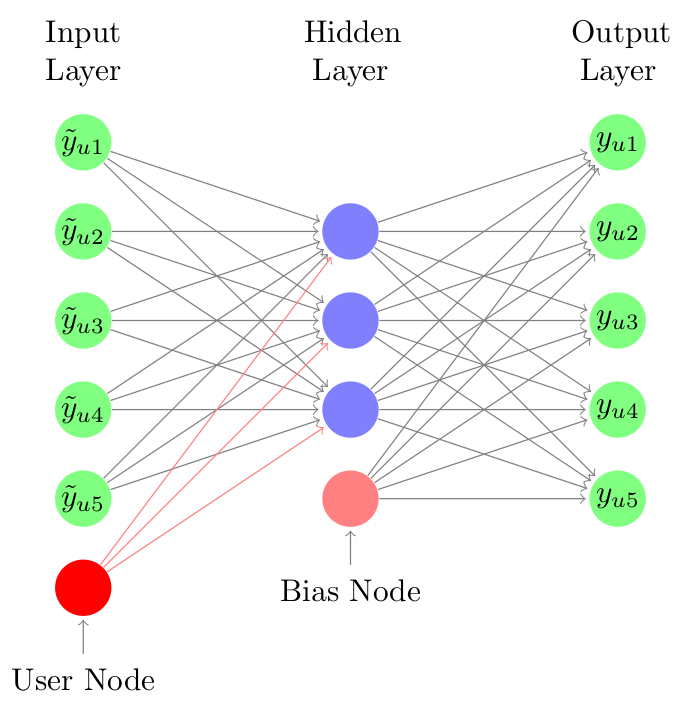}
	\caption{A sample CDAE illustration for a user \textit{u} \cite{wu2016}}
	\label{figure:cdae}
\end{figure}

CDAE, shown in Figure \ref{figure:cdae} assumes that whatever user-item interactions are a corrupted version of the user's full preference set. The model learns latent representations of corrupted user-item preferences that can best reconstruct the full input, recovering co-preference patterns. It uses an additional user node on the input and bias node beside the hidden layer.

\subsubsection{Collaborative Recurrent Autoencoder (CRAE)}
TODO: 

CRAE [Wang et. al, 2016]
Collaborative Recurrent Autoencoder
Encodes text (e.g. movie plot, review)
Autoencoding with RNNs
- Encoder-decoder architecture
- The input is corrupted by replacing words with a deisgnated
BLANK token
CDL model + text encoding simultaneously
- Joint learning

[Wang et. al, 2016] H. Wang, X. Shi, DY. Yeung: Collaborative Recurrent Autoencoder: Recommend while Learning to Fill in the Blanks. Advances in Neural Information
Processing Systems (NIPS 2016)

\subsection{Neural collaborative filtering}

TODO: Summarize from \cite{he2017}

%Code: https://github.com/hexiangnan/neural_collaborative_filtering

\subsubsection{Other Deep CF methods}

Coevolving features [Dai et. al, 2016]
- Users' taste and items' audiences change over time (e.g. forum discussions)
- User/item features depend on time
- User/item features are composed of
-- Time drift vector
-- Self evolution
-- Co-evolution with items/users
-- Interaction vector
- Feature vectors are learned by RNNs

Product Neural Network (PNN) [Qu et. al, 2016]
- For CTR estimation
- Embedded features
- Pairwise layer: all pairwise combination of embedded features
-- Like Factorization Machines
-- Outer/inner product of feature vectors or both
- Several fully connected layers

 CF-NADE [Zheng et. al, 2016] \cite{zheng2016autoregressive}
- Neural Autoregressive Collaborative Filtering
- User events reference (0/1) + confidence (based on occurence)
- Reconstructs some of the user events based on others (not the full set)
-- Random ordering of user events
-- Reconstruct the preference i, based on preferences and confidences up to i-1
- Loss is weighted by confidences
(ver resumo docs) See also http://tech.hulu.com/blog/2016/08/01/cfnade.html
